# Supplementary material for: Evaluating and Enhancing Out-of-Domain Generalization of Task-Oriented Dialog Systems for Task Completion without Turn-level Dialog Annotations
Source: arXiv:2502.13310 source file (2025-02-18)
Supplement: Supplementary file 3 [file appendix_multidomain.tex]

\section{Results to Carry Information from Domain One to Next in Multi-domain Dialogs}
\label{sec:multi_dom_api}

Table~\ref{tab:multi_api_mixed_results} presents the results for Carry Information from Domain One to Next in Multi-domain Dialogs. 
For this setting, we only have results on the SGD and KETOD datasets. We can see that for the key metric, Full API Accuracy, {\opt} achieves the best results across both datasets. {\opt} also achieves the highest scores for the Parameter Names Accuracy and Parameter Values Accuracy metrics as well. However, for the API Invoke Accuracy and API Method Accuracy, on some settings, {\flan} outperforms {\opt}.
Upon comparing the key metric, Full API Accuracy, of single domain results from Table~\ref{tab:api_results} with that of Multi-domain Dialogs, we can see that the performance of the models is better in the Multi-domain dialogs. A possible explanation of this could be that a bulk of the multi-domain dialogs contain common and generic domains like \texttt{Events}, \texttt{Restaurants}, and \texttt{Hotels}.
The dataset contains a lot of example dialogs from these domains, which in turn could have been the reason behind the improved performance. 

We can see that apart from the API Invoke Accuracy and API Method Accuracy, {\opt} is the model that produces the best results for the remaining metrics across both results. {\flan} is the second best performing model, and also achieves best results on the two metrics mentioned before. A notable observation on the key metric, Full Api Accuracy, is that the performance for mixed domain settings is in between that of the seen and unseen domain settings. This is the expected result, as mixed domains contain domains from both seen and unseen domains.

\section{Example Dialogs with Responses from All Models}
\label{sec:example_dialogs}
% Table~\ref{tab:rest_dialog} shows an example dialog in the Restaurant domain. It contains the turn id, user utterance, gold response, \gptt response, and {\flan} response. Texts highlighted in red outlines the portions where the system response by a model is incorrect and green highlights the correct parts.

% Table~\ref{tab:multi_domain_dialog} shows an example multi-domain dialog in the Buses and RideShare domain. Model utterances in red mark the mistakes made and green highlights the correct parts. We can see that \gptt has a common mistake of making an API Call before confirming with the user, whereas {\flan} does not have such an issue. Also, we can see that the responses of \gptt are longer and more descriptive, whereas {\flan} produces short and succint responses, similar to the gold standards.

Table~\ref{tab:rest_dialog} shows an example dialog in the Restaurant domain and Table~\ref{tab:multi_domain_dialog} shows an example multi-domain dialog in the Buses and \texttt{RideShare} domain. The table contains the turn id, user utterance, gold response, {\gptt}, {\gptf}, {\gpt}, {\flan}, and {\opt} response. Text highlighted in red outlines the portions where the system response by a model is incorrect and green highlights the correct parts. Texts highlighted in orange indicate that the model is partially correct and is missing some information. Texts highlighted in yellow indicate that the system response seems like a valid response but is incorrect because the gold standard is expecting a different response. 

From the example dialogs, we can see that {\gptt} and {\gptf} has a common mistake of making an API Call without confirming with the user, whereas {\oursys} models do not make this mistake. Also, we can see that the responses of {\gptt} and {\gptf} are longer and more descriptive, whereas {\oursys} models produce succinct responses, similar to the gold standards. This observation indicates that {\oursys} was able to pick up the text generation style of the gold standard, which is an important aspect for TOD systems.

We can see that {\gpt} hallucinates and makes up information on its own, but {\flan} and {\opt} do not suffer from hallucination as much. For the API call task, all the models face similar problems of missing certain parameters and in the multi-domain setting, the models fail to adapt to the slots of the new domain. For response generation, on turns 1 in Table~\ref{tab:multi_domain_dialog}, we can see the request sub-task challenge as discussed in Section~\ref{sec:response_generation}, where the gold standard expects a certain slot but the models request a different slot. Another observation from turn 2 of that dialog is that the gold standard expects the model to request 3 slots, but the {\oursys} models are only asking about a single slot. A reason for this could be that there fewer turns where the gold standard expects multiple slots to be requested, so the models picked this pattern and asked about one slot.

On turn 4 from Table~\ref{tab:rest_dialog}, we can see that {\gpt} only mentioned that the restaurant was booked but did not mention the cuisine of the restaurant, whereas all other models did not make this mistake. Similar examples exist on a few other turns, where {\gpt} misses important information.

\begin{figure*}
   \centering
   \includegraphics[width=0.95\linewidth]{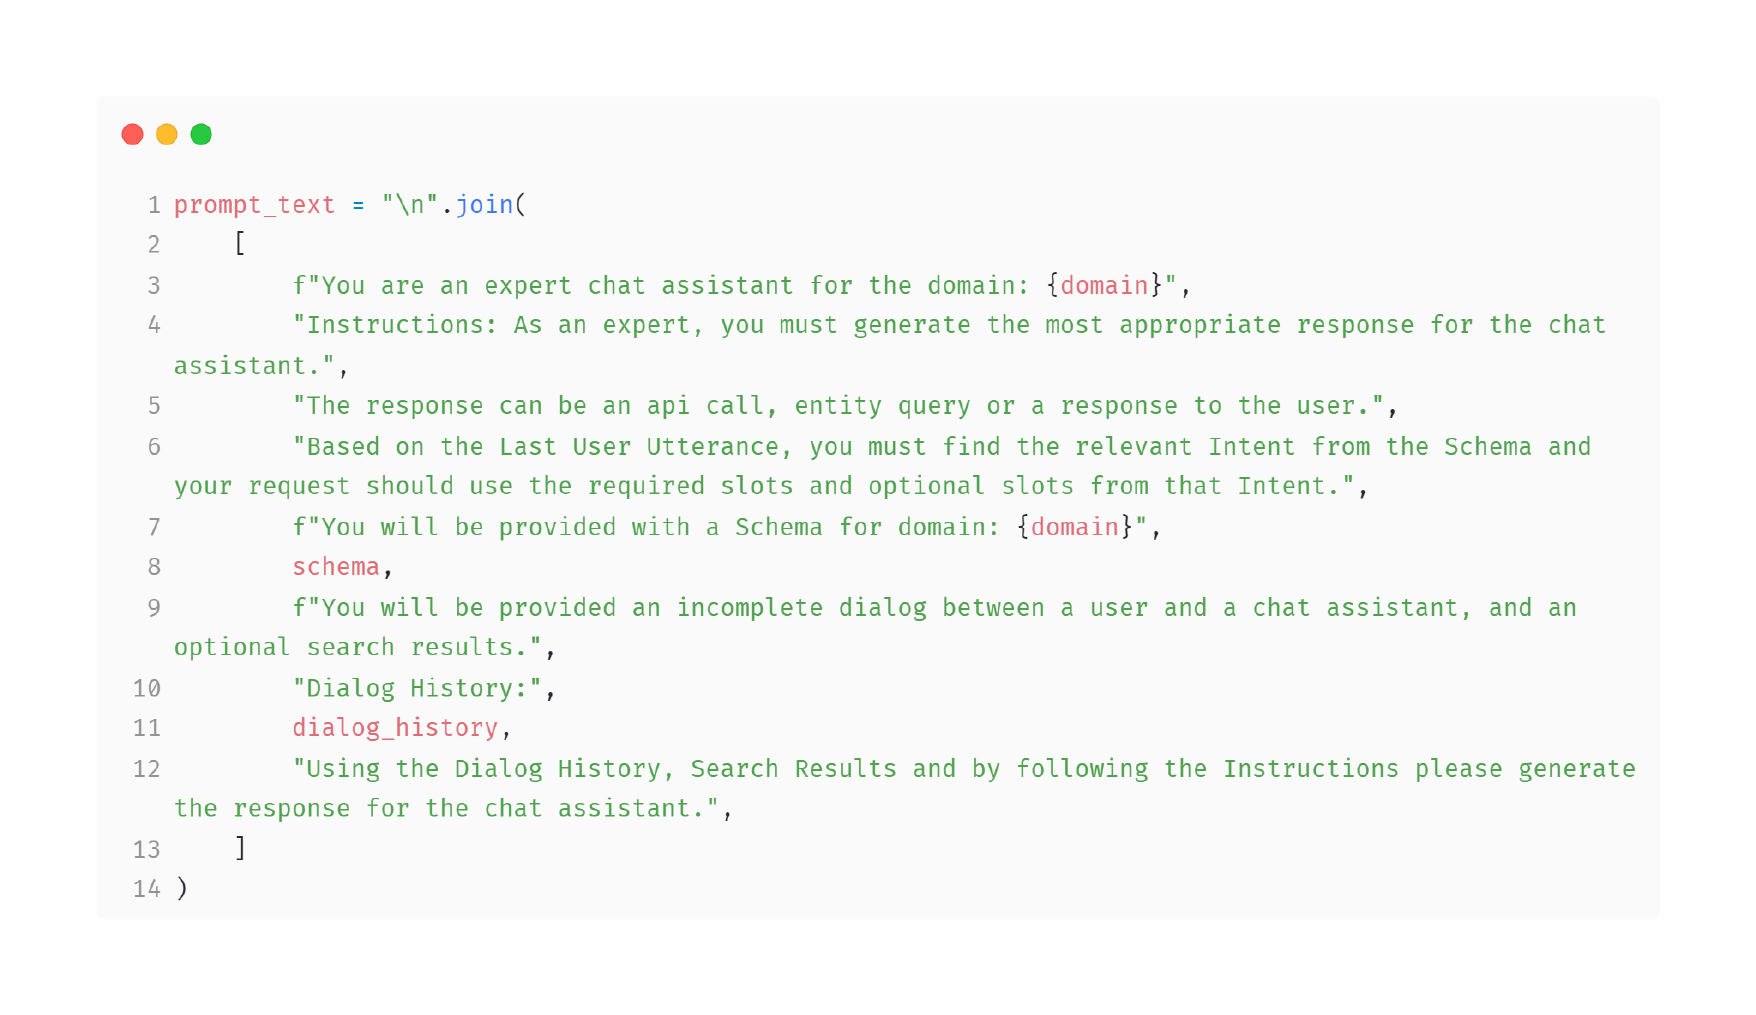}
   
   \caption{
       Template used to generate the prompt for fine-tuning {\oursys}.
   }
   
   \label{fig:finetuning_template}
\end{figure*}

\begin{figure*}
   \centering
   \includegraphics[width=0.95\linewidth]{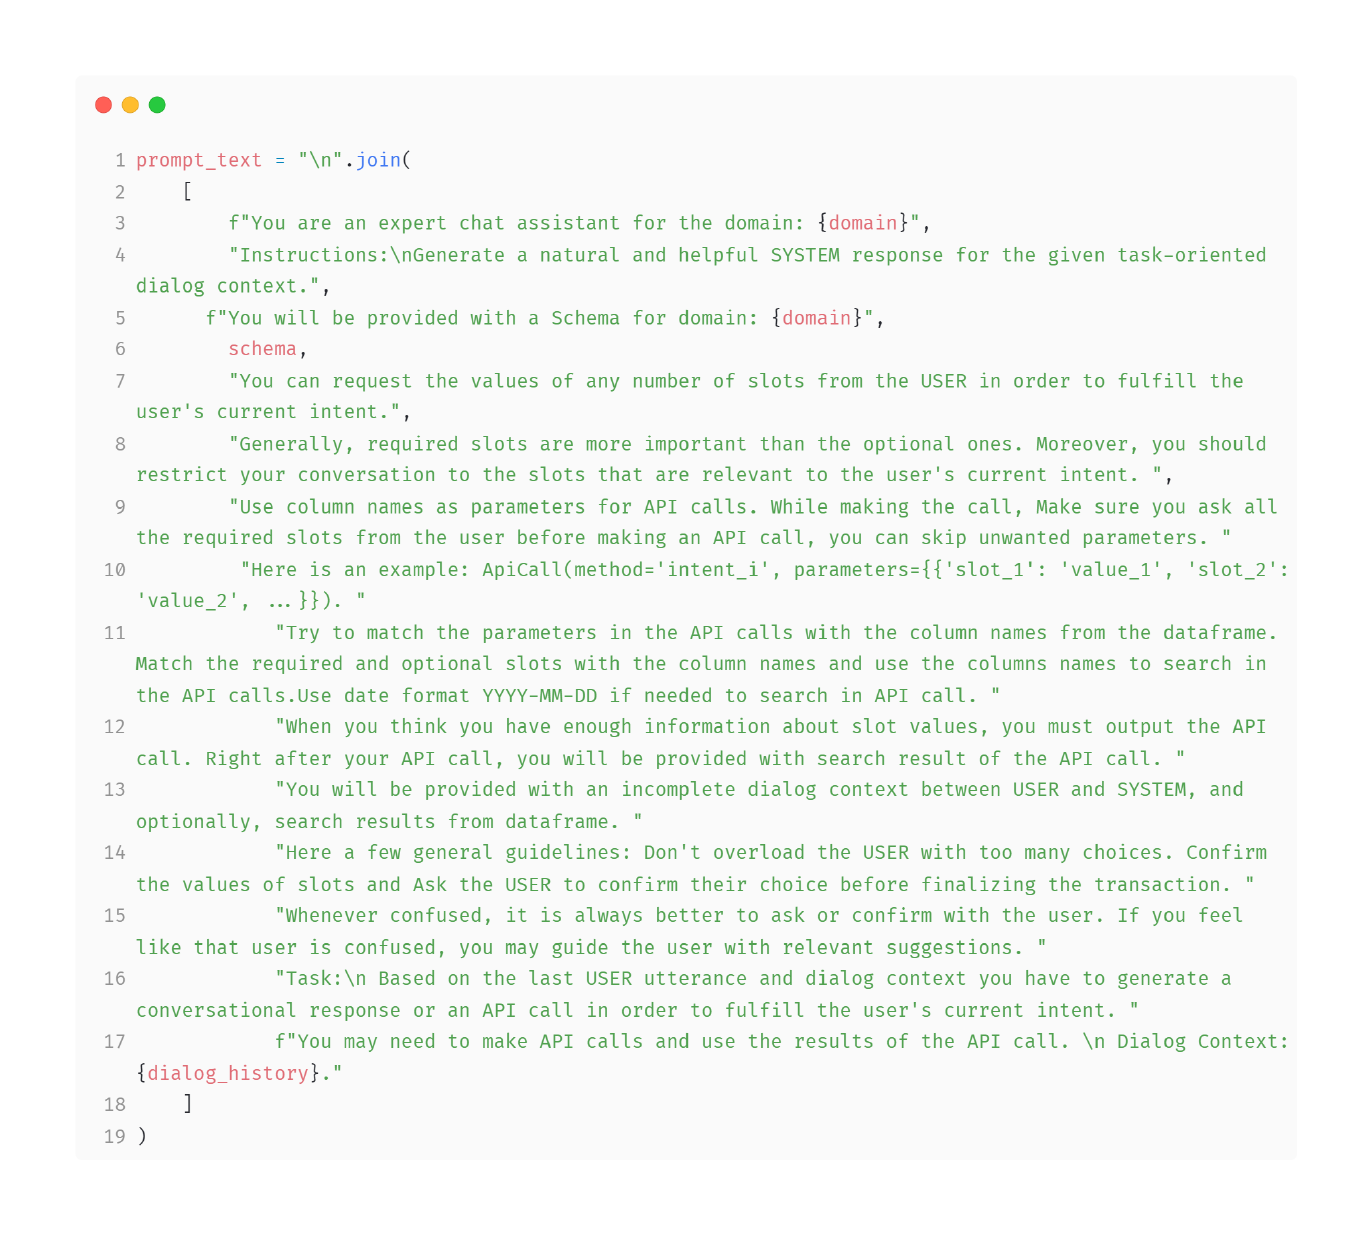}
   \caption{
       Template used to generate the prompt for OpenAI's GPT Models. 
   }
   
   \label{fig:chatgpt_template}
\end{figure*}

\begin{table*}[!t]
    \centering
    \small
    \begin{adjustbox}{max width=\textwidth}
        \begin{tabular}{|c|c|c|c|c| R c|c|c|c|}
            \hline
    \multirow{2}{*}{\textbf{Dataset}}&\multirow{2}{*}{\textbf{Model}} & \multicolumn{4}{R}{\textbf{Overall Response (BLEU-4)}} & \multicolumn{4}{c|}{\textbf{Overall Response (GLEU-4)}}  \\ \cline{3-10}
    & & \textbf{all}  & \textbf{seen} & \textbf{unseen} & \textbf{mixed} & \textbf{all}  & \textbf{seen} & \textbf{unseen} & \textbf{mixed} \\ \hline
    \multirow{4}{*}{SGD}&{\gptt} & 0.0397& 0.0422 & 0.0363 & 0.043
    &  0.0555& 0.0570 & 0.0522 & 0.0589
    \\ 
    &\gpt& 0.2276& 0.2423 & 0.2095 & 0.2436
    &  0.2240& 0.2430 & 0.2060 & 0.2395
    \\ 
    &\flan& \underline{0.2680}& \underline{0.2980} & \underline{0.2500} & \underline{0.2790}
    &  \underline{0.2610}& \underline{0.2960} & \underline{0.2440} & \underline{0.2721}
    \\ 
    &\opt& \textbf{0.3063}& \textbf{0.3311} & \textbf{0.2896} & \textbf{0.3174}
    &  \textbf{0.2996}& \textbf{0.3210} & \textbf{0.2841} & \textbf{0.3115} 
 \\  \hline
    
    % KETOD
    \multirow{4}{*}{KETOD}&{\gptt} &0.0397& 0.0412 & 0.0334 & 0.0438
    & 0.0554& 0.0563 & 0.0494 & 0.0601
    \\ 
    &\gpt&0.1509& 0.1756 & 0.1224 & 0.1507
    & 0.1552& 0.1751 & 0.1303 & 0.1568
    \\ 
    &\flan& \underline{0.2130}  & \underline{0.2503} & \underline{0.1794} & \underline{0.2040}
    & \underline{0.2091} & \underline{0.2408} & \underline{0.1825} & \underline{0.2000}
    \\ 
    &\opt&\textbf{0.2680}  & \textbf{0.2994} & \textbf{0.2371} & \textbf{0.2559}
    & \textbf{0.2534} & \textbf{0.2860} & \textbf{0.2248} & \textbf{0.2446}
 \\  \hline

    % BITOD
        \multirow{4}{*}{BiToD}&{\gptt} &0.0646  & 0.0646 & - & -
    & 0.0760 & 0.0760 & - & -
    \\ 
    &\gpt&\underline{0.3466}  & \underline{0.3466} & - & -
    & \underline{0.3016} & \underline{0.3016} & - & -
    \\ 
    &\flan& 0.3159  & 0.3159 & - & -
    & 0.2640 & 0.2640 & - & -
    \\ 
    &\opt&\textbf{0.4143}& \textbf{0.4143} & - & -
    & \textbf{0.3803}& \textbf{0.3803} & - & -
 \\  \hline
    
        \end{tabular}
    \end{adjustbox}
    \caption{Overall Response Generation: BLEU \& GLEU scores for system generations with additional mixed domain setting.}
    \label{tab:response_gleu_mixed}
    % \vspace{-15pt}
\end{table*}

\begin{table*}[!t]
    \centering
    \small
    \begin{adjustbox}{max width=\textwidth}
        \begin{tabular}{|c|c|c|c|c| R c|c|c|c|}
            \hline
    \multirow{2}{*}{\textbf{Dataset}}&\multirow{2}{*}{\textbf{Model}} & \multicolumn{4}{R}{\textbf{Inform (BLEU-4)}} & \multicolumn{4}{c|}{\textbf{Inform (GLEU-4)}}  \\ \cline{3-10}
    & & \textbf{all}  & \textbf{seen} & \textbf{unseen} & \textbf{mixed} & \textbf{all}  & \textbf{seen} & \textbf{unseen} & \textbf{mixed} \\ \hline
    \multirow{4}{*}{SGD}&{\gptt} &0.1047& 0.0998 & 0.1012 & 0.1094
    & 0.1563& 0.1505 & 0.1523 & 0.1616
    \\ 
    &\gpt& 0.2737& 0.3022& 0.2479 & 0.2913
    &  0.3644& 0.3880& 0.3421 & 0.3799
    \\ 
    &\flan& \underline{0.2991}& \underline{0.3064} & \underline{0.2872} & \underline{0.3099}
    &  \underline{0.3879}& \underline{0.3960} & \underline{0.3775} & \underline{0.3968}
    \\ 
    &\opt&\textbf{0.3334}& \textbf{0.3499} & \textbf{0.3190} & \textbf{0.3431}
    & \textbf{0.4199}& \textbf{0.4322} & \textbf{0.4092} & \textbf{0.4271}
 \\  \hline
    
    % KETOD
    \multirow{4}{*}{KETOD}&{\gptt} &0.0943& 0.0801 & 0.0958 & 0.1108
    & 0.1439& 0.1337 & 0.1428 & 0.1578
    \\ 
    &\gpt& 0.1734& 0.1843 & 0.1498 & 0.1817
    &  0.2565& 0.2717 & 0.2336 & 0.2587
    \\ 
    &\flan&\underline{0.2311}& \underline{0.2435} & \underline{0.2120} & \underline{0.2335}
    & \underline{0.3100}& \underline{0.3243} & \underline{0.2897} & \underline{0.3112}
    \\
    &\opt & \textbf{0.2968} & \textbf{0.2981} & \textbf{0.3034} & \textbf{0.2889}
    &  \textbf{0.3726}& \textbf{0.3776} & \textbf{0.3746} & \textbf{0.3646} 
 \\  \hline

    % BITOD
        \multirow{4}{*}{BiToD}&{\gptt}& 0.2589& 0.2589 & - &-
    &  0.3092& 0.3092 & - &-
    \\ 
    &\gpt& \underline{0.5226}& \underline{0.5226} & - & -
    &  \underline{0.5682}& \underline{0.5682} & - & -
    \\ 
    &\flan& 0.4795& 0.4795 & - & -
    &  0.5389& 0.5389 & - & -
    \\ 
    &\opt& \textbf{0.5248}& \textbf{0.5248} & - & -
    &  \textbf{0.5900}& \textbf{0.5900} & - & -
 \\  \hline
    
        \end{tabular}
    \end{adjustbox}
    \caption{BLEU \& GLEU scores for inform sub-task of response generation task, with additional mixed domain setting.}
    \label{tab:inform_gleu_mixed}
    % \vspace{-15pt}
\end{table*}

\begin{table*}[!t]
    \centering
    \small
    \begin{adjustbox}{max width=\textwidth}
        \begin{tabular}{|c|c|c|c|c| R c|c|c|c|}
            \hline
    \multirow{2}{*}{\textbf{Dataset}}&\multirow{2}{*}{\textbf{Model}} & \multicolumn{4}{R}{\textbf{Request (BLEU-4)}} & \multicolumn{4}{c|}{\textbf{Request (GLEU-4)}}  \\ \cline{3-10}
    & & \textbf{all}  & \textbf{seen} & \textbf{unseen} & \textbf{mixed} & \textbf{all}  & \textbf{seen} & \textbf{unseen} & \textbf{mixed} \\ \hline
    \multirow{4}{*}{SGD}& {\gptt} &0.0057 & 0.0046 & 0.0056 & 0.0060
    & 0.0337 & 0.0299 & 0.0343 & 0.0343
    \\ 
    &\gpt& 0.0616& 0.0659 & 0.0630 & 0.0588
    &  0.1387& 0.1453 & 0.1403 & 0.1353
    \\ 
    &\flan&\underline{0.0657}& \underline{0.0742} & \underline{0.0698} & \underline{0.0582}
    & \underline{0.1552}& \underline{0.1687} & \underline{0.1586} & \underline{0.1477}
    \\ 
    &\opt& \textbf{0.0836}& \textbf{0.0928} & \textbf{0.0793} & \textbf{0.0868}
    &  \textbf{0.1767}& \textbf{0.1870} & \textbf{0.1721} & \textbf{0.1803}
 \\  \hline
    
    % KETOD
    \multirow{4}{*}{KETOD}&{\gptt} &0.0033& 0.0036 & 0.0037 & 0.0026
    & 0.0305& 0.0285 & 0.0332 & 0.0300
    \\ 
    
    &\gpt& 0.0140& 0.0193& 0.0073 & 0.0148
    &  0.0649& 0.0750& 0.0561 & 0.0620
    \\ 
    
    &\flan&\underline{0.0587}& \underline{0.0781} & \underline{0.0430} & \underline{0.0521}
    & \underline{0.1440}& \underline{0.1707} & \underline{0.1256} & \textbf{0.1315}
    \\ 
    
    &\opt& \textbf{0.0640}& \textbf{0.0851}& \textbf{0.0509} & \textbf{0.0526}
    &  \textbf{0.1475}& \textbf{0.1742}& \textbf{0.1339} & \underline{0.1301}
    
 \\  \hline

    % BITOD
        \multirow{4}{*}{BiToD}&{\gptt} &0.0011& 0.0011& - & -
    & 0.0219& 0.0219& - & -
    \\ 
    &\gpt& \underline{0.0323}& \underline{0.0323} & - & -
    &  \underline{0.1035}& \underline{0.1035} & - & -
    \\ 
    &\flan&0.0256& 0.0256 & - & -
    & 0.0811& 0.0811 & - & -
    \\ 
    &\opt& \textbf{0.0476}& \textbf{0.0476} & - & -
    &  \textbf{0.1260}& \textbf{0.1260} & - & -
    
 \\  \hline
    
        \end{tabular}
    \end{adjustbox}
    \caption{BLEU \& GLEU scores for request sub-task of response generation task, with additional mixed domain setting.}
    \label{tab:seeking_information_gleu_mixed}
    % \vspace{-15pt}
\end{table*}

\begin{table*}[!t]
    \centering
    \begin{adjustbox}{max width=\textwidth}
        \begin{tabular}{|c|c|c|c|c|c|c|c|c|c|c|c|c|c|}
            \hline
            \multirow{2}{*}{\textbf{Metric}} & \multirow{2}{*}{\textbf{Model}} & \multicolumn{4}{c|}{\textbf{SGD}} & \multicolumn{4}{c|}{\textbf{KETOD}} & \multicolumn{4}{c|}{\textbf{BiToD}} \\ \cline{3-14}
            & & \textbf{all} & \textbf{seen} & \textbf{unseen} & \textbf{mixed} & \textbf{all} & \textbf{seen} & \textbf{unseen} & \textbf{mixed} & \textbf{all} & \textbf{seen} & \textbf{unseen} & \textbf{mixed} \\ \hline

            \multirow{2}{*}{API} 
            & \gptt & 68.42 & 69.16 & 68.01 & 68.65 & 64.57 & 65.10 & 63.22 & 65.06 & 44.59 & 44.59 & - & - \\ 
            \multirow{2}{*}{Invoke} & \gpt & 90.51 & 97.66 & 86.21 & 93.11 & 78.83 & 80.87 & 73.56 & 80.75 & 93.46 & 93.46 & - & - \\ 
            \multirow{2}{*}{Accuracy} & \flan & \textbf{98.65} & \underline{99.61} & \textbf{98.24} & \textbf{98.84} & \textbf{90.45} & \textbf{89.93} & \textbf{90.34} & \textbf{91.09} & \textbf{98.48} & \textbf{98.48} & - & - \\ 
            & \opt & \underline{97.02} & \textbf{99.84} & \underline{95.81} & \underline{97.59} & \underline{82.22} & \underline{81.38} & \underline{84.14} & \underline{81.64} & \underline{97.36} & \underline{97.36} & - & - \\ 

            \hline
            \multirow{2}{*}{API} 
            & \gptt & 66.09 & 66.98 & 65.38 & 66.57 & 62.12 & 62.08 & 62.99 & 61.50 & 08.31 & 08.31 & - & - \\ 
            \multirow{2}{*}{Method} & \gpt & 78.62 & 96.26 & 71.42 & 81.80 & 71.48 & 78.36 & 62.53 & 71.12 & 87.34 & 87.34 & - & - \\ 
            \multirow{2}{*}{Accuracy} & \flan & \textbf{96.84} & \underline{99.61} & \textbf{95.23} & \textbf{97.81} & \textbf{89.07} & \textbf{89.93} & \textbf{86.67} & \textbf{90.02} & \textbf{93.07} & \textbf{93.07} & - & - \\ 
            & \opt & \underline{94.74} & \textbf{99.84} & \underline{92.13} & \underline{96.17} & \underline{78.45} & \underline{80.87} & \underline{77.70} & \underline{76.47} & \underline{92.70} & \underline{92.70} & - & - \\ 

            \hline
            \multirow{2}{*}{Parameter} 
            & \gptt & 67.24 & 64.84 & 68.38 & 66.65 & 63.47 & 61.17 & 67.11 & 63.08 & 04.53 & 04.53 & - & - \\ 
            \multirow{2}{*}{Name} & \gpt & 60.65 & 92.07 & 49.52 & 64.69 & 57.02 & 72.98 & 39.60 & 53.57 & 86.29 & 86.29 & - & - \\ 
            \multirow{2}{*}{Accuracy} & \flan & \underline{79.71} & \underline{96.97} & \underline{74.58} & \underline{86.68} & \underline{78.62} & \textbf{88.92} & \underline{67.93} & \textbf{75.97} & \underline{90.76} & \underline{90.76} & - & - \\ 
            & \opt & \textbf{90.41} & \textbf{98.19} & \textbf{87.86} & \textbf{91.21} & \textbf{79.50} & \underline{83.85} & \textbf{78.94} & \underline{75.30} & \textbf{92.32} & \textbf{92.32} & - & - \\ 

            \hline
            \multirow{2}{*}{Parameter} 
            & \gptt & 61.37 & 60.56 & 61.72 & 61.21 & 57.64 & 56.03 & 60.30 & 57.28 & 04.15 & 04.15 & - & - \\ 
            \multirow{2}{*}{Values} & \gpt & 58.64 & 91.24 & 46.98 & 62.95 & 55.46 & 71.83 & 37.73 & 51.83 & 86.10 & 86.10 & - & - \\ 
            \multirow{2}{*}{Accuracy} & \flan & \underline{76.03} & \underline{94.04} & \underline{70.43} & \underline{84.51} & \underline{76.52} & \textbf{87.94} & \underline{65.28} & \textbf{73.09} & \underline{85.47} & \underline{85.47} & - & - \\ 
            & \opt & \textbf{87.70} & \textbf{97.91} & \textbf{84.02} & \textbf{89.08} & \textbf{77.43} & \underline{83.46} & \textbf{75.87} & \underline{72.22} & \textbf{92.17} & \textbf{92.17} & - & - \\ 

            \hline
            \multirow{2}{*}{Full} 
            & \gptt & 33.32 & 32.63 & 28.52 & 38.06 & 29.59 & 30.54 & 23.45 & 33.33 & 02.36 & 02.36 & - & - \\ 
            \multirow{2}{*}{Api} & \gpt & 36.72 & 83.41 & 19.40 & 43.48 & 36.75 & 59.56 & 10.80 & 32.62 & 83.19 & 83.19 & - & - \\ 
            \multirow{2}{*}{Accuracy} & \flan & \underline{56.64} & \underline{89.49} & \underline{41.96} & \underline{63.79} & \textbf{59.42} & \textbf{83.72} & \underline{35.86} & \textbf{51.87} & \underline{73.79} & \underline{73.79} & - & - \\ 
            & \opt & \textbf{63.81} & \textbf{90.97} & \textbf{51.98} & \textbf{69.42} & \underline{57.35} & \underline{77.18} & \textbf{39.54} & \underline{50.09} & \textbf{91.11} & \textbf{91.11} & - & - \\

            \hline
        \end{tabular}
    \end{adjustbox}
    \vspace{-6pt}
    \caption{Detailed results for API calls across different metrics and datasets along with mixed domain.}
    \label{tab:api_results_mixed}
    \vspace{-12pt}
\end{table*}

\begin{table*}[!t]
    \centering
    \begin{adjustbox}{max width=\textwidth}
        \begin{tabular}{|c|c|c|c|c|R c|c|c |R c|c|c|c|}
            \hline
            \multirow{2}{*}{\textbf{Metric}} & \multirow{2}{*}{\textbf{Model}} & \multicolumn{4}{R}{\textbf{SGD}} & \multicolumn{4}{R}{\textbf{KETOD}} & \multicolumn{4}{c|}{\textbf{BiToD}} \\ \cline{3-14}
            & & \textbf{all} & \textbf{seen} & \textbf{unseen} & \textbf{mixed} & \textbf{all} & \textbf{seen} & \textbf{unseen}  & \textbf{mixed} & \textbf{all} & \textbf{seen} & \textbf{unseen}  & \textbf{mixed} \\ \hline
            
            \multirow{2}{*}{Api} 
            & \gptt & 68.34 & 73.42 & 67.77 & 68.12 & 62.05 & 61.05 & 66.00 & 61.20 & 29.47 & 29.47 & - & - \\ 
            \multirow{2}{*}{Invoke} & \gpt & 92.32 & 97.75 & 89.06 & 93.95 & 84.02 & 85.26 & 81.33 & 84.15 & \textbf{99.90} & \textbf{99.90} & - & - \\ 
            \multirow{2}{*}{Accuracy} & \flan & \textbf{98.80} & \underline{98.87} & \textbf{98.42} & \textbf{99.00} & \textbf{89.01} & \textbf{88.07} & \underline{90.00} & \textbf{89.34} 
            & 95.14 & 95.14 & - & -  \\ 
            & \opt & \underline{96.32} & \textbf{99.55} & \underline{94.98}  & \underline{96.87} & \underline{88.64} & \underline{87.72} & \textbf{92.67} & \underline{87.70} & \underline{99.31} & \underline{99.31} & - & - \\ 

            \hline
            \multirow{2}{*}{Api} 
            & \gptt & 65.94 & 72.07 & 64.80 & 66.01 & 60.05 & 58.60 & 66.67 & 58.47 & 12.23 & 12.23 & - & - \\ 
            \multirow{2}{*}{Method} & \gpt & 81.24 & 97.07 & 73.76 & 84.57 & 78.65 & 83.51 & 68.67 & 78.96 & 91.29 & 91.29 & - & - \\ 
            \multirow{2}{*}{Accuracy} & \flan & \textbf{96.94} & \underline{98.87} & \textbf{95.05}& \textbf{97.97} 
            & \textbf{87.02} & \textbf{88.07} & \underline{83.33} & \textbf{87.70} & \underline{91.53} & \underline{91.53} & - & - \\ 
            & \opt & \underline{93.87} & \textbf{99.55} & \underline{90.80} & \underline{95.33} & \underline{86.27} & \underline{87.72} & \textbf{86.00} & \underline{85.25} & \textbf{92.41} & \textbf{92.41} & - & - \\ 

            \hline
            \multirow{2}{*}{Parameter} 
            & \gptt & 65.85 & 68.99 & 64.65 & 66.31 & 60.07 & 58.10 & \underline{64.27} & 59.89 & 09.17 & 09.17 & - & - \\ 
            \multirow{2}{*}{Names} & \gpt & 58.23 & 95.61 & 44.97 & 63.01 & 61.22 & 79.28 & 35.37 & 57.76 & \underline{90.40} & \underline{90.40} & - & - \\ 
            \multirow{2}{*}{Accuracy} & \flan & \underline{77.31} & \underline{98.47} & \underline{72.96} & \underline{83.18} 
            & \underline{75.18} & \underline{87.11} & 62.96 & \underline{70.89} & 88.43 & 88.43 & - & - \\ 
            & \opt & \textbf{89.30} & \textbf{99.19} & \textbf{86.38} & \textbf{90.16} & \textbf{82.17} & \textbf{87.78} & \textbf{79.44} & \textbf{78.92} & \textbf{92.01} & \textbf{92.01} & - & -  \\ 

            \hline
            \multirow{2}{*}{Parameter} 
            & \gptt & 61.39 & 65.19 & 58.88 & 62.69 & 56.18 & 55.20 & 57.80 & 56.28 & 08.60 & 08.60 & - & - \\ 
            \multirow{2}{*}{Values} & \gpt & 56.46 & 94.52 & 42.59 & 61.60 & 59.44 & 77.53 & 33.22 & 56.09 & \underline{90.29} & \underline{90.29} & - & - \\ 
            \multirow{2}{*}{Accuracy} & \flan & \underline{73.77} & \underline{96.32} & \underline{68.36} & \underline{81.18}
            & \underline{73.16} & \underline{85.87} & \underline{59.72}& \underline{68.77} & 82.90 & 82.90 & - & - \\ 
            & \opt & \textbf{86.61} & \textbf{98.77} & \textbf{82.10} & \textbf{88.30}& \textbf{79.75} & \textbf{87.16} & \textbf{75.55} & \textbf{75.70} & \textbf{91.95} & \textbf{91.95} & - & - \\ 

            \hline
            \multirow{2}{*}{Full} 
            & \gptt & 38.62 & 40.77 & 33.66 & 41.83 & 34.08 & 36.84 & 26.67 & 34.97 & 03.55 & 03.55 & - & - \\ 
            \multirow{2}{*}{Api} & \gpt & 36.31 & 87.39 & 19.32 & 42.07 & 43.07 & 68.07 & 12.00 & 36.34 & \underline{88.14} & \underline{88.14} & - & - \\ 
            \multirow{2}{*}{Accuracy} & \flan & \underline{50.72} & \underline{92.12} & \underline{35.09} & \underline{56.39} 
            & \underline{56.30} & \underline{82.46} & \underline{30.00}& \underline{46.72} & 72.79 & 72.79 & -& -  \\ 
            & \opt & \textbf{61.13} & \textbf{96.40} & \textbf{46.91} & \textbf{66.85}& \textbf{60.55} & \textbf{83.16} & \textbf{36.67} & \textbf{52.73} & \textbf{91.38} & \textbf{91.38} & - & - \\ 

            \hline
        \end{tabular}
    \end{adjustbox}
    \caption{Results for carry information from domain one to next in multi-domain dialogs along with mixed domains.}
    \label{tab:multi_api_mixed_results}
\end{table*}
