# Supplementary material for: Evaluating and Enhancing Out-of-Domain Generalization of Task-Oriented Dialog Systems for Task Completion without Turn-level Dialog Annotations
Source: arXiv:2502.13310 source file (2025-02-18)
Supplement: Supplementary file 5 [file appendix_dialogs_old.tex]

% \begin{table*}
%     \centering
%     \begin{adjustbox}{max width=0.95\textwidth}
%         \begin{tabular}{r|p{0.9\textwidth}}
\onecolumn
\begin{longtblr}[
  caption = {Dialog from Restaurant domain in SGD dataset. Dialog id 1\_00001},
  label = {tab:rest_dialog},
]{
  colspec = {r|X[5]},
  rowhead = 0,
  hlines,
  row{even} = {},
  row{1} = {},
} 
            Turn & 1 \\ 
            User & Can you book a table for me at the Ancient Szechuan for the 11th of this month at 11:30 am?  \\ 
            Gold & In which city are you trying to book the table? \\ 
            \gptt & \color{BrickRed} Sure, I can help you with that. Just to confirm, you would like to make a reservation at Ancient Szechuan for the 11th of this month at 11:30 am, is that correct? \\ 
            \gptf &\color{ForestGreen}  Could you please confirm the location where you'd like to book the table at Ancient Szechuan? Additionally, how many seats will you need for the reservation?
 \\
            \gpt & \color{BrickRed} Sure, please confirm you'd like a table for 2 at Ancient Szechuan in San Jose at 11:30 am on March 11th.\\ 
            \flan & \color{ForestGreen} Sure, where are you located?  \\ 
            \opt & \color{ForestGreen} Sure, what city is that in? \\ 

            
            Turn & 2 \\ 
            User &  Can you book a table at the Butterfly restaurant in San Francisco?  \\ 
            Gold & Please confirm that you need a table for 2 at the Butterfly Restaurant in San Francisco at 11:30 am on March 11th. \\ 
            \gptt & \color{BrickRed} ApiCall(method=`ReserveRestaurant', parameters=`restaurant\_name': `Butterfly', `location': `San Francisco')\\ 
            \gptf &  \color{ForestGreen} Could you please confirm the date and time you would like to reserve the table at Butterfly Restaurant in San Francisco? Also, how many seats will you need?
\\
            \gpt & \color{ForestGreen} Please confirm that you want to book a table for 2 at the Butterfly restaurant in San Francisco. The reservation is for March 11th at 11:30 am.
 \\ 
            \flan & \color{ForestGreen} Please confirm the following details: Booking a table for 2 at Butterfly Restaurant in San Francisco on March 11th at 11:30 am. \\ 
            \opt & \color{ForestGreen} Please confirm that you want me to book a table for 2 at the Butterfly Restaurant in San Francisco on March 11th at 11:30 am. \\ 
            
            Turn & 3 \\ 
            Gold & ApiCall(method=`ReserveRestaurant', parameters= `date': `2019-03-11', `location': `San Francisco', `number\_of\_seats': `2',`restaurant\_name': `Butterfly Restaurant', `time': `11:30' )\\ 
            \gptt & ApiCall(\color{BrickRed} method=`FindRestaurants', parameters=`category': `All', `location': `San Francisco') \\ 
            \gptf & \color{BrickRed} Great, the reservation is nearly complete. As for the cuisine, the Butterfly Restaurant mainly offers modern American cuisine with a focus on seasonal ingredients. Would you like to proceed with the booking for March 11th at 11:30 am at the Butterfly Restaurant?
 \\
            \gpt & ApiCall(method=`ReserveRestaurant', \color{BrickRed}parameters=`city': `San Francisco', \color{ForestGreen}`date': `2019-03-11', \color{BrickRed}`party\_name': `Luxury Szechuan', \color{ForestGreen}`time': `11:30')

\\ 
            \flan & \color{ForestGreen} ApiCall(method=`ReserveRestaurant', parameters= `location': `San Francisco', `date': `2019-03-11', \color{BrickRed} `party\_size': `2', \color{ForestGreen}`restaurant\_name': `Butterfly Restaurant', `time': `11:30' )\  \\ 
            \opt & \color{Orange} ApiCall(method=`ReserveRestaurant', parameters=`location': `San Francisco', `date': `2019-03-11', `restaurant\_name': `Butterfly Restaurant', `time': `11:30') \\ 


            
            Turn & 4 \\ 
            User & That's perfect. What cuisine do they offer?  \\ 
            Gold & \color{ForestGreen} Your table has been booked successfully and they serve Asian cuisine. \\ 
            \gptt & \color{ForestGreen}The Butterfly Restaurant in San Francisco offers Asian cuisine. \color{BrickRed}Would you like me to proceed with booking a table for you at the Butterfly Restaurant in San Francisco for 2 people on March 11th at 11:30 am?\\ 
            \gptf & \color{ForestGreen} Your reservation at Butterfly Restaurant in San Francisco is confirmed for 2 people on March 11th at 11:30 am. The restaurant is located at 33 The Embarcadero and specializes in Asian cuisine. They also offer vegetarian options and have a moderate price range. Is there anything else I can assist you with today?
  \\
            \gpt & \color{Orange} Your table is booked.
\\
            \flan & \color{ForestGreen}Your reservation has been made. They serve Asian food. \\ 
            \opt & \color{ForestGreen} I've successfully booked your table. They offer Asian cuisine. \\ 

            
            Turn & 5 \\ 
            User & Can you get me the user rating of the restaurant? Is it expensive? \\ 
            Gold & Their prices are moderate and they have a user rating of 4.0. \\ 
            \gptt & \color{ForestGreen}The user rating of the Butterfly Restaurant is 4.00. It is considered to be in the moderate price range.\\ 
            \gptf & \color{ForestGreen} The Butterfly Restaurant in San Francisco has a user rating of 4.00 out of 5, and it falls within a moderate price range. Is there anything else you would like to know or another way I can assist you today?
\\
            \gpt & \color{ForestGreen}The restaurant is rated 4.0. The price range is moderate.
 \\
            \flan & \color{ForestGreen}The rating is 4.0 and the price range is moderate. \\ 
            \opt & \color{ForestGreen}The price range is moderate and the rating is 4.0. \\ 

                        
            Turn & 6 \\ 
            User & Thanks a bunch! \\ 
            Gold & Is there anything else I can do for you? \\ 
            \gptt & \color{ForestGreen} You're welcome! If you have any more questions or need further assistance, feel free to ask. Enjoy your dining experience at Butterfly Restaurant!\\ 
            \gptf & \color{ForestGreen} You're welcome! If you need any more assistance or another reservation, just let me know. Enjoy your meal at Butterfly Restaurant!
 \\
            \gpt & \color{ForestGreen} Is there anything else I can help you with?\\
            \flan & \color{ForestGreen} Can I help you with anything else? \\ 
            \opt & \color{ForestGreen} Is there anything else I can do for you? \\ 

                
            Turn & 7 \\ 
            User & No. Thank you. That's all I need. \\ 
            Gold & Have a great day! \\ 
            \gptt & \color{ForestGreen}You're welcome! If you need any more assistance in the future, feel free to reach out. Have a great day!\\ 
            \gptf & \color{ForestGreen} You're welcome! If you need any more assistance in the future, feel free to ask. Have a wonderful day!
\\
            \gpt & \color{ForestGreen}Have a great day!
\\
            \flan & \color{ForestGreen}Have a great day! \\ 
            \opt & \color{ForestGreen}My pleasure. Have a great day! \\ 

            
%         \end{tabular}
%     \end{adjustbox}
%     \caption{Dialog from Restaurant domain in SGD dataset. Dialog id 1\_00001}
%     \label{tab:rest_dialog}
% \end{table*}

\end{longtblr}

% Switch back to two-column mode
\twocolumn

%12_00066


% 1200006
\onecolumn
\begin{longtblr}[
  caption = {Multi domain dialog example from the Buses and RideShare domain in SGD dataset. Dialog id 12\_00006},
  label = {tab:multi_domain_dialog},
]{
  colspec = {r|X[5]},
  rowhead = 0,
  hlines,
  row{even} = {},
  row{1} = {},
} 
    Turn & 1 \\ 
    User & I need bus tickets. \\ 
    Gold & How many tickets? \\ 
    \gptt & \color{myyellow}Sure, I can help you with booking bus tickets. Can you please provide me with the following information: from which city, to which city, and on what date do you need the bus tickets? \\ 
    \gptf & \color{ForestGreen} Great, I can help you with that! Could you please provide me with the departure city, destination city, and the date you plan to travel? Additionally, it would be helpful to know how many passengers will be traveling and if you have a preferred bus category.
 \\
    \gpt & \color{myyellow}What time do you want to leave?
\\
    \flan & \color{myyellow} Where are you going? \\ 
    \opt & \color{myyellow} Where are you departing from? \\

    
    Turn & 2 \\ 
    User & For three people. \\
    Gold & When would you like to leave and at what time? Where are you heading to? \\   
    \gptt & \color{ForestGreen}Sure! I will need some more information to help you with the bus tickets. Can you please provide me with the departure city, destination city, and the date of travel?\\ 
    \gptf & \color{ForestGreen} Great! For which cities and what is the departure date for the bus tickets you need for three people?
\\
    \gpt & \color{orange}What time do you want to leave?
\\
    \flan & \color{orange} Where are you going? \\ 
    \opt & \color{orange} Where are you departing from? \\
    
    Turn & 3 \\ 
    User & I want to leave for Anaheim on the 11th of March at afternoon 3:30. \\ 
    Gold & Where would you be leaving from?  \\ 
    \gptt & \color{BrickRed} ApiCall(method=`FindBus', parameters={`from\_city': `current\_city', `to\_city': `Anaheim', `departure\_date': `2023-03-11', `num\_passengers': 3}) \\ 
    \gptf & \color{ForestGreen} Could you please confirm the city you'll be departing from to travel to Anaheim?
 \\
    \gpt & \color{BrickRed}You want 3 tickets on the bus leaving at 3:30 pm on March 11th at Anaheim.
\\
    \flan & \color{ForestGreen}Where are you leaving from? \\ 
    \opt & \color{ForestGreen} Where are you leaving from? \\
    
    Turn & 4 \\ 
    User & I would be leaving LA.  \\ 
    Gold & You would like tickets for 3 on a bus leaving Los Angeles for Anaheim on March 11th at 3:30 pm with no extra luggage. \\ 
    \gptt & \color{BrickRed} System: ApiCall(method=`BuyBusTicket', parameters={`from\_city': `LA', `to\_city': `Anaheim', `departure\_date': `2023-03-11', `departure\_time': `15:30', `num\_passengers': `3'}) \\ 
    \gptf & \color{BrickRed} ApiCall(method=`BuyBusTicket', parameters=\{`from\_city': `LA', `to\_city': `Anaheim', `departure\_date': `2023-03-11', `departure\_time': `15:30', `num\_passengers': `3'\})
 \\
    \gpt & \color{orange} You would like 3 tickets on a bus leaving at 3:30 pm on March 11th at 3:30 pm on the bus leaving from Los Angeles.
\\
    \flan & \color{ForestGreen} Please confirm: 3 tickets for the bus leaving Los Angeles on March 11th at 3:30 pm to Anaheim. \\ 
    \opt & \color{ForestGreen} You want 3 tickets for a bus from Los Angeles to Anaheim on March 11th at 3:30 pm? \\


    Turn & 5 \\ 
    Gold & ApiCall(method=`BuyBusTicket', parameters= `additional\_luggage': `False', `departure\_date': `2019-03-11', `departure\_time': `15:30', `from\_city': `Los Angeles', `num\_passengers': `3', `to\_city': `Anaheim' ) \\ 
    \gptt & \color{BrickRed} In order to get accurate information on the number of stops and the specific station the bus will be leaving from, it is best to contact the bus company directly. Would you like me to assist you in finding contact information for the bus company or would you like to handle it on your own? \\ 
    \gptf & \color{BrickRed}It looks like you're ready to purchase the bus tickets. However, I'll need to check the details of the bus trip including the number of stops and departure station. I'll proceed with that now.
\color{ForestGreen}ApiCall(method=`BuyBusTicket', parameters=\{`from\_city': `Los Angeles', `to\_city': `Anaheim', `departure\_date': `2023-03-11', `departure\_time': `15:30', `num\_passengers': 3\})
 \\
    \gpt & \color{orange}ApiCall(method=`BuyBusTicket', parameters=`departure\_date': `2019-03-11', `departure\_time': `15:30', `destination': `Anaheim', \color{BrickRed}`origin': `Los Angeles') \\
    \flan & \color{orange} ApiCall(method=`BuyBusTicket', parameters=`departure\_date': `2019-03-11', `departure\_time': `15:30', \color{ForestGreen}`to\_city': `Anaheim', `number\_of\_passengers': `3' ) \\ 
    \opt & \color{orange}ApiCall(method='BuyBusTicket', parameters={'from\_city': 'Los Angeles', 'departure\_date': '2019-03-11', 'departure\_time': '15:30', 'to\_city': 'Anaheim', 'num\_passengers': '3'}) \\
    
    Turn & 6 \\ 
    User & That would be fine. How many stops are there and which station would it be leaving from?  \\ 
    Gold & It is a direct bus and it would be leaving North Hollywood Station. I have bought the tickets. \\ 
    \gptt & \color{BrickRed} In order to get accurate information on the number of stops and the specific station the bus will be leaving from, it is best to contact the bus company directly. Would you like me to assist you in finding contact information for the bus company or would you like to handle it on your own? \\ 
    \gptf & \color{orange} The bus leaves from North Hollywood Station and arrives at Anaheim Bus Station. It's a direct bus with no stops. The total price for all three tickets will be \$39. Would you like to proceed with the purchase?
 \\
    \gpt & \color{ForestGreen}I have bought the tickets. There is a direct bus leaving at 3:30 pm and there are 0 stops.
 \\
    \flan & \color{ForestGreen} Your tickets have been confirmed. The bus will be leaving from North Hollywood Station and there are \color{BrickRed}10 stops. \\ 
    \opt & \color{ForestGreen}I have confirmed the tickets. There are only \color{BrickRed}1 stop and \color{ForestGreen}it leaves from North Hollywood Station.\\

    
    Turn & 7 \\ 
    User & I would need a nice SUV rental car in Anaheim on the 12th of this month. \\ 
    Gold & What time would you like to pick up the car and till when would you like it? \\ 
    \gptt & \color{BrickRed} The bus you're looking for is a direct route from Los Angeles to Anaheim on March 11th at 3:30 pm. The bus will be leaving from North Hollywood Station. Would you like to proceed with booking these tickets? \\ 
    \gptf & \color{ForestGreen} In order to assist you with the SUV rental in Anaheim, could you please provide the pick-up and drop-off times, as well as let me know if you'd like to add insurance to your booking?
\\
    \gpt & \color{BrickRed}You would like to pick up the car at Anaheim Bus Station on March 12th?
\\
    \flan &  \color{orange} What time would you like to pick it up? \\ 
    \opt & \color{orange} What time would you like to pick it up? \\

    Turn & 8 \\ 
    Gold & ApiCall(method=`GetCarsAvailable', parameters=`car\_type': `SUV', `city': `Anaheim', `end\_date': `2019-03-13', `pickup\_time': `12:00',`start\_date': `2019-03-12' )\\ 
    \gptt & \color{ForestGreen} ApiCall(method=`GetCarsAvailable', parameters={`city': `Anaheim', `start\_date': `2019-03-12', `pickup\_time': `12:00', `end\_date': `2019-03-13', `car\_type': `SUV'}) \\ 
    \gptf & \color{BrickRed} Thank you for the information. Could you also specify which type of SUV you would prefer for your rental in Anaheim, or should I proceed with any available SUV?
 \\
    \gpt & \color{ForestGreen}ApiCall(method=`GetCarsAvailable', parameters=\color{BrickRed}`dropoff\_date': `2019-03-13', `pickup\_city': `Anaheim', `pickup\_date': `2019-03-12', \color{ForestGreen}`pickup\_time': `12:00')\\
    \flan & \color{orange}ApiCall(method=`GetCarsAvailable', parameters=`car\_type': `Suv', `city': `Anaheim', `pickup\_date': `2019-03-12', `pickup\_time': `12:00' ) \\ 
    \opt & \color{ForestGreen}ApiCall(method=`GetCarsAvailable', parameters=\color{BrickRed}`car\_type': `Full-size', \color{ForestGreen}`start\_date': `2019-03-12', `end\_date': `2019-03-13', \color{BrickRed}`pickup\_location': `Anaheim', `start\_time': `12:00') \\

    Turn & 9 \\ 
    User & I want to pick it up at 12 in the afternoon and drop it off on the 13th of this month. \\ 
    Gold & There is a nice SUV Dacia Duster available at Anaheim Intermodal Center.  \\ 
    \gptt & \color{BrickRed} When would you like to pick up the SUV rental car in Anaheim on the 12th of this month? \\ 
    \gptf & \color{ForestGreen} We have an SUV available for your dates in Anaheim. It's a Dacia Duster, and you can pick it up at the Anaheim Intermodal Center at 12:00 pm on the 12th of March, and drop it off on the 13th of March. The rental price is \$43.00 per day. Would you like to go ahead and reserve this car? Additionally, do you require insurance for the rental?
 \\
    \gpt & \color{ForestGreen}There is a nice car at Anaheim Intermodal Center for pickup on March 12th. It is a SUV and it is a nice car.
\\
    \flan & \color{ForestGreen}There is a nice car available at Anaheim Intermodal Center on March 12th. It is a Dacia Duster. \\ 
    \opt & \color{BrickRed}There are 5 cars available.\color{ForestGreen} There is a nice Dacia Duster that is available at Anaheim Intermodal Center and it is a SUV. It would be available on March 12th. \\

    Turn & 10 \\ 
    User & How much does it cost daily? \\ 
    Gold & It cost \$43.00 a day.  \\ 
    \gptt & The SUV rental car you requested, a Dacia Duster, is available for pick up at the Anaheim Intermodal Center at 12:00 on March 12th. The rental period will be until 12:00 on March 13th, and the \color{ForestGreen}price per day is \$43.00. I will proceed with reserving this car for you. \\ 
\gptf &  \color{ForestGreen} The Dacia Duster SUV is available for a daily rate of \$43.00. Would you like to proceed with the reservation?
\\
    \gpt & \color{ForestGreen}The cost is \$43.00.
 \\

    \flan & \color{ForestGreen}It would cost \$43.00 per day. \\ 
    \opt & \color{ForestGreen}It costs \$43.00 daily. \\

    Turn & 11 \\ 
    User &  Go ahead and reserve the car \\ 
    Gold &  Would you like to add insurance? \\ 
    \gptt & \color{BrickRed}The SUV Dacia Duster in Anaheim Intermodal Center costs \$43.00 per day. \\ 
  \gptf & \color{ForestGreen} Would you like to add insurance to your car reservation?
 \\
    \gpt & \color{BrickRed}You would like to pick up a nice car at Anaheim Intermodal Center on March 12th at 12 pm and drop it off on March 13th?
\\

    \flan & \color{BrickRed} You would like to pick up a nice car from Anaheim Intermodal Center on March 12th at 12 pm and drop it off on March 13th. Is this correct? \color{ForestGreen} You would like to add insurance to the car. \\ 
    \opt & \color{BrickRed} You want a full-size car and would like to pick it up at Anaheim Intermodal Center on March 12th at 12 pm and drop it off on March 13th. Is that right? \\


    Turn & 12 \\ 
    User & I don't need it. \\ 
    Gold & You would like to pick up a SUV at Anaheim Intermodal Center on March 12th at 12 pm and drop it off on March 13th  \\ 
    \gptt & \color{BrickRed} ApiCall(method=`ReserveCar', parameters={`car\_type': `SUV', `city': `Anaheim', `end\_date': `2019-03-13', `pickup\_location': `Anaheim Intermodal Center', `pickup\_time': `12:00', `start\_date': `2019-03-12', `add\_insurance': `False'}) \\ 
    \gptf & \color{BrickRed} ApiCall(method=`ReserveCar', parameters={`pickup\_location': `Anaheim Intermodal Center', `start\_date': `2019-03-12', `pickup\_time': `12:00', `end\_date': `2019-03-13', `car\_type': `SUV', `add\_insurance': `False'})

 \\
    \gpt & \color{BrickRed}Is there anything else I can help you with?
\\
    \flan & \color{BrickRed} Is there anything else I can help you with? \\ 
    \opt & \color{orange}Would you like to pick up the car at Anaheim Intermodal Center on March 12th at 12 pm? \\


    Turn & 13 \\ 
    Gold & ApiCall(method=`ReserveCar', parameters=`add\_insurance': `False', `car\_type': `SUV', `end\_date': `2019-03-13', `pickup\_location': `Anaheim Intermodal Center', `pickup\_time': `12:00',`start\_date': `2019-03-12' ) \\ 
    \gptt & \color{ForestGreen} ApiCall(method=`ReserveCar', parameters={`car\_type': `SUV', `city': `Anaheim', `end\_date': `2019-03-13', `pickup\_location': `Anaheim Intermodal Center', `pickup\_time': `12:00', `start\_date': `2019-03-12', `add\_insurance': `False'}) \\ 
    \gptf & \color{ForestGreen} ApiCall(method=`ReserveCar', parameters={`pickup\_location': `Anaheim Intermodal Center', `start\_date': `2019-03-12', `pickup\_time': `12:00', `end\_date': `2019-03-13', `car\_type': `SUV', `add\_insurance': `False'})

 \\
    \gpt & \color{ForestGreen}ApiCall(method=`ReserveCar', parameters=`car\_type': `SUV', \color{BrickRed}`dropoff\_date': `2019-03-13', `pickup\_date': `2019-03-12', \color{ForestGreen}`pickup\_location': `Anaheim Intermodal Center', `pickup\_time': `12:00')\\
    \flan & \color{ForestGreen}ApiCall(method=`ReserveCar', parameters=`car\_type': 'SUV', \color{BrickRed}`dropoff\_date': `2019-03-13', \color{ForestGreen}`pickup\_location': `Anaheim Intermodal Center', \color{BrickRed}`pickup\_date': `2019-03-12', \color{ForestGreen}`pickup\_time': `12:00' ) \\ 
    \opt & \color{ForestGreen}ApiCall(method='ReserveCar', parameters={'car\_type': 'SUV', 'end\_date': '2019-03-13', 'pickup\_location': 'Anaheim Intermodal Center', 'pickup\_time': '12:00', \color{BrickRed}'end\_date': '2019-03-13'}) \\


    Turn & 14 \\ 
    User & Yes, that would be great. \\ 
    Gold & I have reserved the car. \\ 
    \gptt & \color{BrickRed} ApiCall(method=`ReserveCar', parameters={`car\_type': `SUV', `pickup\_location': `Anaheim Intermodal Center', `start\_date': `2019-03-12', `end\_date': `2019-03-13', `pickup\_time': `12:00', `add\_insurance': `False'}) \\ 
    \gptf & \color{ForestGreen} Your reservation has been confirmed for the Dacia Duster SUV at Anaheim Intermodal Center. You can pick it up on March 12th at 12:00 PM and return it by March 13th. The cost is \$43.00 per day, and you've chosen not to add insurance. Is there anything else I can assist you with today?
 \\
    \gpt & \color{ForestGreen}I have reserved the car.
\\
    \flan &\color{ForestGreen} Your car has been reserved. \\ 
    \opt & \color{ForestGreen}I have reserved the car. \\


    Turn & 15 \\ 
    User & Thanks a lot. \\ 
    Gold & Anything else you need? \\ 
    \gptt & \color{BrickRed} System: You would like to pick up a SUV at Anaheim Intermodal Center on March 12th at 12 pm and drop it off on March 13th. Your reservation for a Dacia Duster SUV at \$43.00 per day has been confirmed. \\ 
    \gptf &  \color{ForestGreen} You're welcome! If you need any more assistance or have further questions, feel free to ask. Have a great trip!
\\
    \gpt &\color{ForestGreen} Is there anything else?
\\
    \flan & \color{ForestGreen}Is there anything else I can help you with? \\ 
    \opt &\color{ForestGreen} Is there anything else I can help you with? \\


    Turn & 16 \\ 
    User & No, thanks a lot \\ 
    Gold & Enjoy your day. \\ 
    \gptt & \color{ForestGreen}You're welcome! If you need any more assistance or have any other questions, feel free to ask. Have a great day! \\ 
    \gptf & \color{ForestGreen} You're welcome! Have a great trip to Anaheim and enjoy your ride! If you need anything else in the future, just let me know. Safe travels!
 \\
    \gpt & \color{ForestGreen}Enjoy your day.
\\
    \flan & \color{ForestGreen}Have a great day. \\ 
    \opt &\color{ForestGreen} Enjoy your day. \\


\end{longtblr}

% Switch back to two-column mode
\twocolumn
